# Supplementary material for: Incorporating Contact Network Structure in Cluster Randomized Trials
Source: arXiv:1505.00044 source file (2015-04-30)

$\gamma=0$

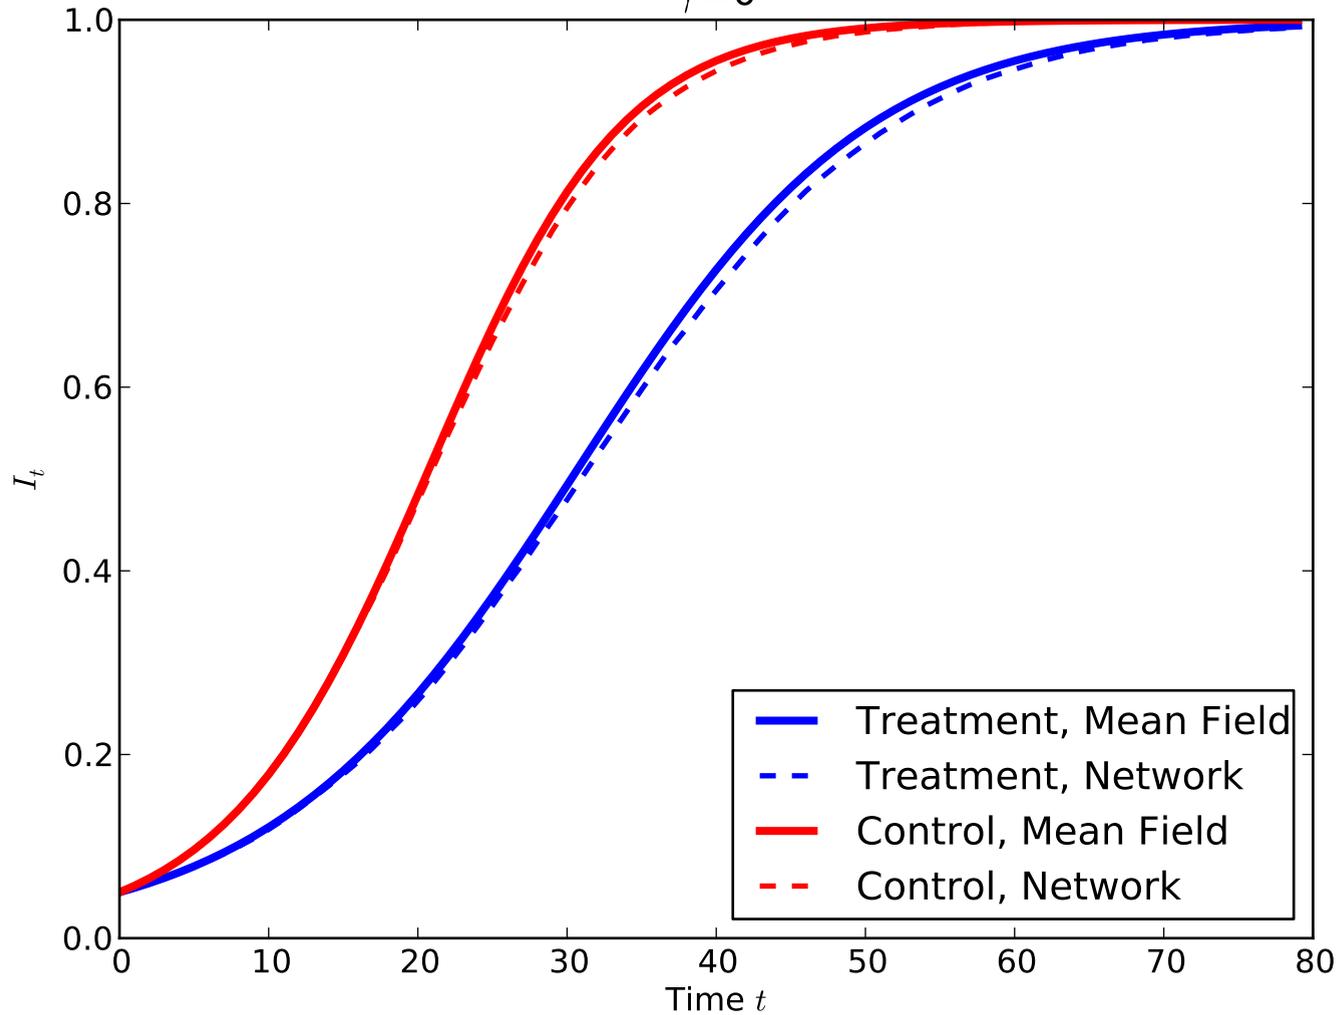

$\gamma=0.1$

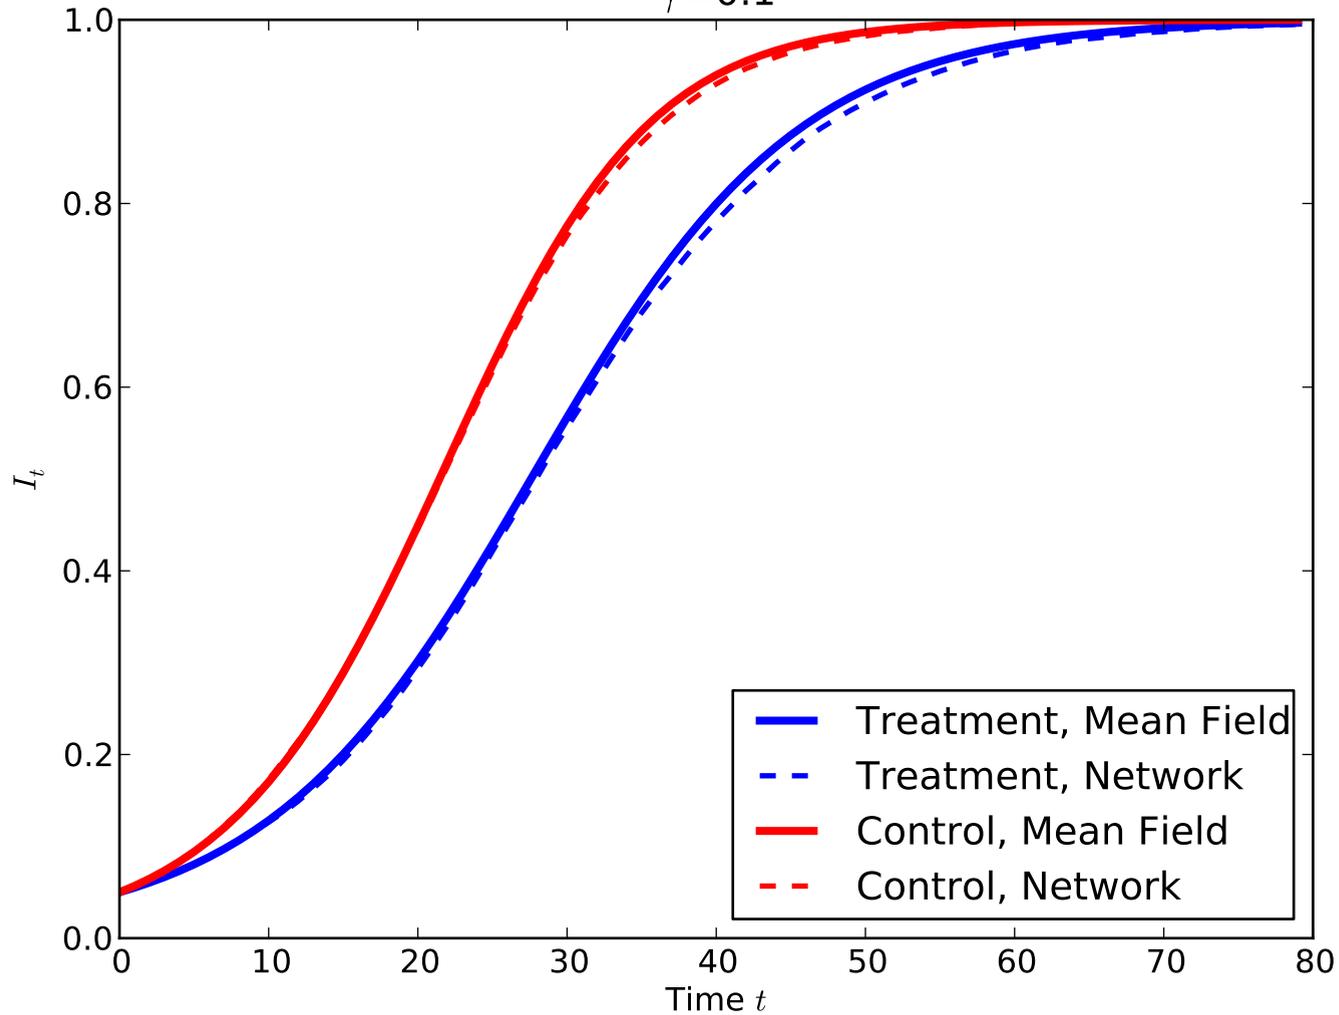

$\gamma=0.2$

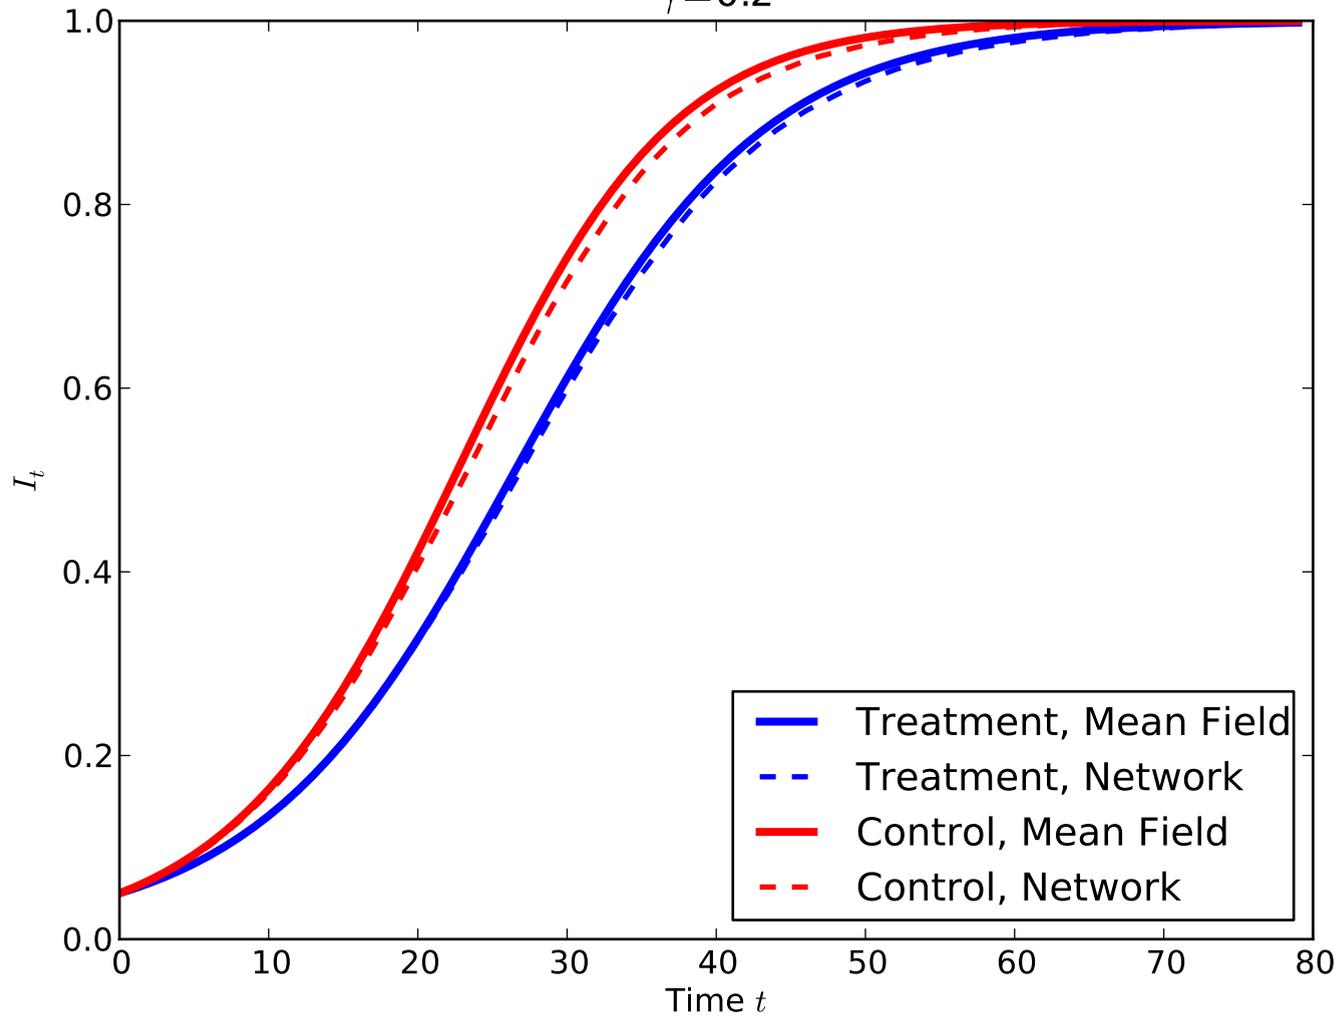

$\gamma=1$

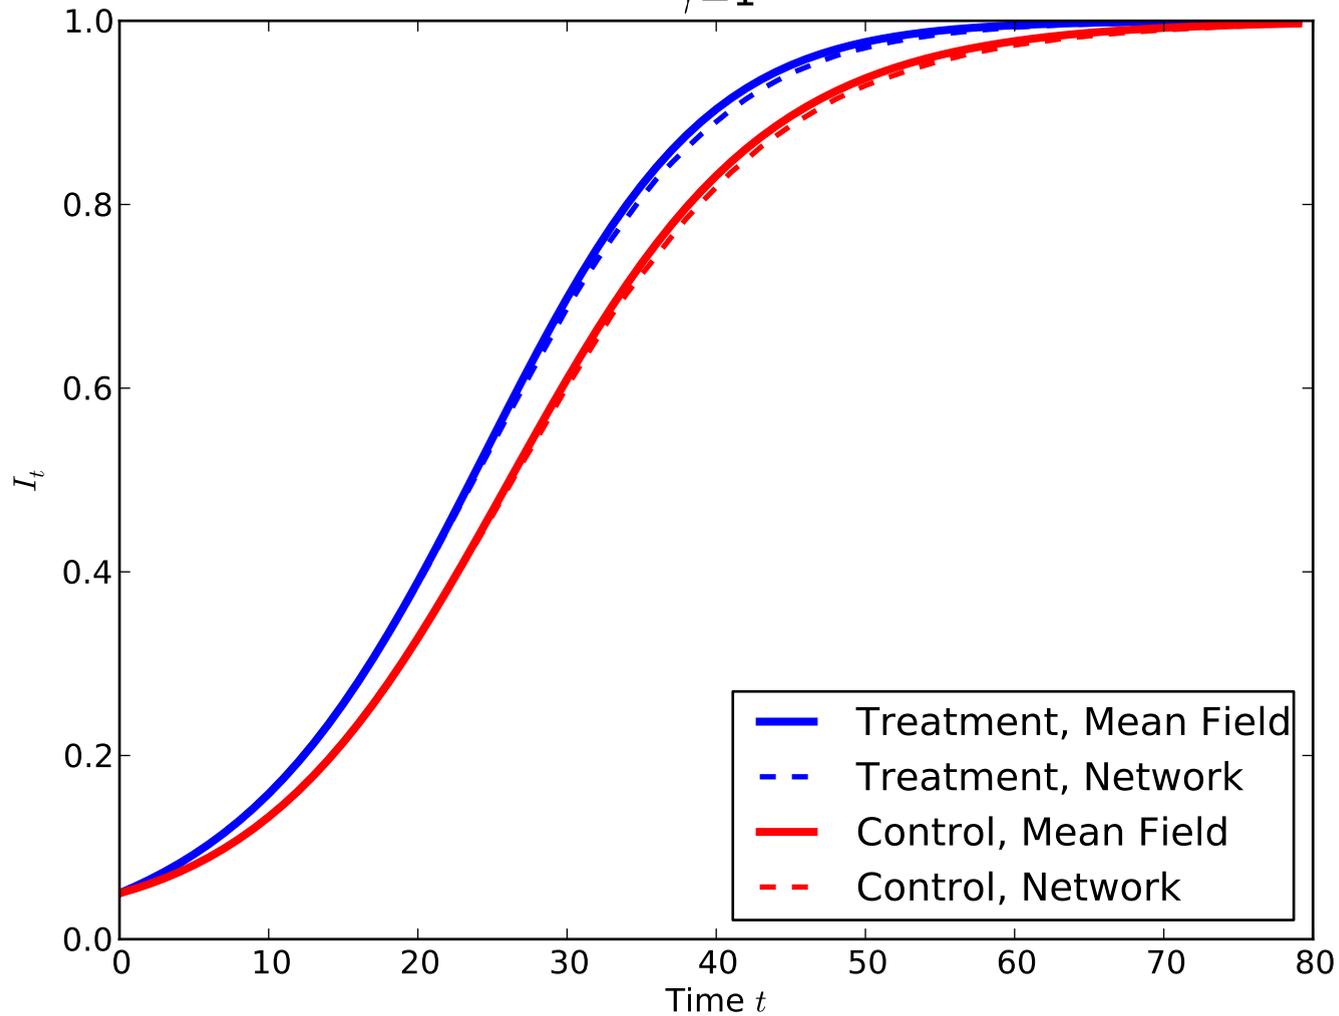

Supplement: Supplementary file 1 [file supplementary_figure_1.pdf]
